# Supplementary material for: Environment assisted and environment hampered efficiency at maximum power in a molecular photo cell
Source: arXiv:2003.11564 ancillary file (2020-03-27)
Supplement: Supplementary file 1 [file supplement.pdf]

# Supplementary: Environment assisted and environment hampered efficiency at maximum power in a molecular photo cell\*

Subhajit Sarkar<sup>†</sup> and Yonatan Dubi<sup>‡</sup>

Chemistry Department, Ben-Gurion University, Be'er Sheva 84105, Israel.

(Dated: March 27, 2020)

## I. METHOD AND DETAILS OF CALCULATIONS

We have used the Lindblad master equation to describe the coupling between the system and the environment, which in the Schrödinger's picture is given by,

$$\dot{\rho} = -\frac{i}{\hbar}[H, \rho] + \sum_{\alpha} (V_{\alpha}\rho V_{\alpha}^{\dagger} - \frac{1}{2}\{V_{\alpha}^{\dagger}V_{\alpha}, \rho\}) \quad (1)$$

where  $\rho$  is the density matrix in the Hilbert space,  $\mathcal{H}_{sites} \otimes \mathcal{H}_{ph}$  of the combined electron phonon system. and  $V_{\alpha}$  are a set of Lindblad operators which encode the effects of the coupling to the environment [1–5]. In order to calculate the density matrix at the steady state we focus on the density operator acting on the finite dimensional Hilbert space with  $\mathcal{H}_{sites} = 2^3$  for the effective 3-site model of HPV cell corresponding to the main text. The dimension of the truncated Hilbert space for the Bosonic degrees of freedom is  $\mathcal{H}_{ph} = 6$ , a choice which is the minimum required to leave the results independent of the value of  $\mathcal{H}_{ph}$ . As a result, our Hilbert space dimension is  $N = 2^3 \times 6 (=48)$ . The density matrix, obeying the Lindblad equation therefore, is an  $N \times N$  positive definite matrix with trace one. The standard practice of solving the (1) is to vectorize the  $\rho$  into a  $N^2$  dimension vector. This results in a reformulations of the Lindblad equation into a  $N^2$  dimensional Linear ODE with time independent coefficients ,

$$\dot{\rho} = -\mathcal{L}\rho, \quad (2)$$

$\mathcal{L}$  being the Lindblad super-operator having dimension  $N^2 \times N^2$ . Solving the Lindblad equation for the steady state density matrix  $\rho_{SS}$  then amounts to find the “Null-Space” of the operator  $\mathcal{L}$ , and subsequently reshaping the vector  $\rho_{SS}$  into a matrix of dimension  $N \times N$ . The existence of the “Null-Space” corresponding to the eigenvalue with zero real part is guaranteed by the trace preserving property of the Lindblad equation.

Our next step is to determine the expressions for all the current operators using the conservation of particle occupations numbers  $n_i = \text{Tr}[\hat{n}_i \rho_{SS}]$  at the steady state. We note that in the Schrödinger's picture  $\frac{dn_i}{dt} = 0$  for any number operator  $\hat{n}_i = c_i^{\dagger} c_i$  where  $i = \{D_1, D_2, A\}$ .

Therefore, the rate of change of particle occupation of a particular molecular level relates the net current into and out of that level as,

$$\frac{dn_i}{dt} = \text{Tr}[\hat{J}_i \rho], \quad (3)$$

where  $\hat{J}_i$  is the corresponding current operator, and at the steady state the net current is zero. Our task then is to evaluate the left hand side of the above equation applying the Lindblad equation. Using the cyclic property of the trace operation it is easy to find that,

$$\frac{dn_i}{dt} = \text{Tr}[\{i[H, \hat{n}_i] + \frac{1}{2} \sum_{\alpha} (V_{\alpha}^{\dagger}[\hat{n}_i, V_{\alpha}] + [V_{\alpha}^{\dagger}, \hat{n}_i]V_{\alpha})\}\rho]. \quad (4)$$

At this point it is worthwhile to collect all the Lindblad ‘ $V_{\alpha}$ ’ operators that have been used. From the left electrode to the D-HOMO the Lindblad ‘ $V$ ’ operators are,  $V_{L,+} = \sqrt{\gamma_L f_L (\epsilon_{D_1} - \mu_L)} c_{D_1}^{\dagger}$  for injecting particle into D-HOMO, and  $V_{L,-} = \sqrt{\gamma_L \tilde{f}_L (\epsilon_{D_1} - \mu_L)} c_{D_1}$  for the reverse process with  $\tilde{f} = (1 - f)$ . We set the chemical potential of the left electrode at  $\mu_L = 0$ . The left electrode can be considered to be an electron gas, and so as the right electrode. The Lindblad ‘ $V$ ’ operators between the right electrode and acceptor are given by,  $V_{R,+} = \sqrt{\gamma_R f_R (\epsilon_A - \mu_R)} c_A^{\dagger}$  for creating electron in acceptor and  $V_{R,-} = \sqrt{\gamma_R \tilde{f}_R (\epsilon_A - \mu_R)} c_A$  for the reverse process. We set the chemical potential of the right electrode at  $\mu_R = V$ , i.e., at the Bias voltage. Furthermore in our calculation we set  $\gamma_L = \gamma_R = \gamma = 10^{10} \text{sec}^{-1}$  which is much smaller than the other energy scales in the system validating the use of Lindblad formalism. The radiative and non-radiative  $V$ -operators are given in equations (3) and (4) of the main text. The  $V$ -operator for the Bosonic bath are given by,  $V_{ph,+} = \sqrt{\gamma_{phn} n_B (\Delta\epsilon, T_{ph})} b^{\dagger}$  and  $V_{ph,-} = \sqrt{\gamma_{phn} [n_B (\Delta\epsilon, T_{ph}) + 1]} b$ . Moreover, it is worthwhile to mention the results of a few commutator brackets,  $i[H_e, \hat{n}_{D_1}] = i[H_{e-ph}, \hat{n}_{D_1}] = 0$ ;  $i[H_e, \hat{n}_{D_2}] = -i[H_e, \hat{n}_A] = it(c_{D_2}^{\dagger} c_A - c_A^{\dagger} c_{D_2})$ , and  $i[H_{e-ph}, \hat{n}_{D_2}] = -i[H_{e-ph}, \hat{n}_A] = i\lambda_{e-ph}(bc_{D_2}^{\dagger} c_A - b^{\dagger} c_A^{\dagger} c_{D_2})$ , which are used in obtaining the expression for the current operators below. It is worthwhile to point out that these commutator brackets contribute to the Hamiltonian current. Now, evaluating (4) for D-HOMO it is easy to find that,

\* A footnote to the article title

<sup>†</sup> subhajit@post.bgu.ac.il

<sup>‡</sup> jdubi@bgu.ac.il

$\frac{dn_{D_1}}{dt} = \text{Tr}[(\hat{J}_L - \hat{J}_r - \hat{J}_{nr})\rho]$ , where

$$\begin{aligned}\hat{J}_L &= \gamma_L(f_L(\epsilon_{D_1} - \mu_L) - \hat{n}_{D_1}) \\ \hat{J}_r &= (V_{D_1 \rightarrow D_2}^r)^\dagger V_{D_1 \rightarrow D_2}^r - (V_{D_2 \rightarrow D_1}^r)^\dagger V_{D_2 \rightarrow D_1}^r \\ \hat{J}_{nr} &= (V_{D_1 \rightarrow D_2}^{nr})^\dagger V_{D_1 \rightarrow D_2}^{nr} - (V_{D_2 \rightarrow D_1}^{nr})^\dagger V_{D_2 \rightarrow D_1}^{nr},\end{aligned}\quad (5)$$

and at the steady state  $\frac{dn_{D_1}}{dt} = 0$  renders  $\hat{J}_L = \hat{J}_r + \hat{J}_{nr}$ , where  $\hat{J}_L$  is the current entering into the D-HOMO from the left electrode,  $\hat{J}_{nr}$  is the radiative(non-radiative) part of the current from D-HOMO to D-LUMO. Similarly evaluating (4) for D-LUMO we find,  $\frac{dn_{D_2}}{dt} = \text{Tr}[(\hat{J}_r + \hat{J}_{nr} - \hat{J}_{DA} - \hat{J}_{e-ph})\rho]$ , where

$$\begin{aligned}\hat{J}_{DA} &= -it(c_{D_2}^\dagger c_A - c_A^\dagger c_{D_2}) \\ \hat{J}_{e-ph} &= -i\lambda_{e-ph}(bc_{D_2}^\dagger c_A - b^\dagger c_A^\dagger c_{D_2}),\end{aligned}\quad (6)$$

and  $\hat{J}_r + \hat{J}_{nr} = \hat{J}_{DA} + \hat{J}_{e-ph}$  at the steady state, where  $\hat{J}_{DA}$ ,  $\hat{J}_{e-ph}$  are the pure electronic and e-ph current, respectively, between the D-LUMO and the acceptor. Evaluation of (4) for A-LUMO leads to,

$$\hat{J}_R = -\gamma_R(f_R(\epsilon_A - \mu_R) - \hat{n}_A),\quad (7)$$

where  $\hat{J}_R = \hat{J}_{DA} + \hat{J}_{e-ph}$  at the steady state. In our calculation, the steady state output current is given by,  $J_{out} = -J_R = -\text{Tr}[\hat{J}_R \rho_{SS}]$  which goes into the right electrode. On the other hand the input current is given by the radiative part of the current, i.e.,  $J_{in} = \text{Tr}[\hat{J}_r \rho_{SS}]$  flowing from D-HOMO to D-LUMO. Therefore, the input power is given by,  $P_{in} = (\epsilon_{D_2} - \epsilon_{D_1})J_{in}$  and output power is given by,  $P_{out} = VJ_{out}$ . It is worthwhile to explicitly mention the different particle occupation numbers, viz.,

$$\begin{aligned}n_{D-HOMO} &= \text{Tr}[(c_{D_1}^\dagger c_{D_1})\rho_{SS}] \\ n_{D-LUMO} &= \text{Tr}[(c_{D_2}^\dagger c_{D_2})\rho_{SS}] \\ n_{A-LUMO} &= \text{Tr}[(c_A^\dagger c_A)\rho_{SS}] \\ n_{phn} &= \text{Tr}[(b^\dagger b)\rho_{SS}],\end{aligned}\quad (8)$$

at the steady state. These are evaluated and plotted in the main text on various occasions.

## II. ELECTRON HOPPING DOMINATED TRANSPORT

In this section we compare our model (model 1) of photon and phonon bath involved in the radiative and non-radiative transitions between the D-HOMO and D-LUMO with that of Ref. [6] (model 2). For completeness we rewrite the model considered in Ref. [6], while our model is explained in sec. II of the main text. The full Hamiltonian of the HPV cell is given by  $H$  of the main text and the photon and phonon bath involved in the electronic transitions between D-HOMO and D-LUMO are represented by photon (phonon) Hamiltonian

$H_{pht}(H_{phn})$  and molecule-photon (phonon) interaction Hamiltonian  $H_{M-pht}$  ( $H_{M-phn}$ ) and are given below,

$$\begin{aligned}H_{pht} &= (\epsilon_{D_2} - \epsilon_{D_1})a^\dagger a \\ H_{phn} &= (\epsilon_{D_2} - \epsilon_{D_1})b^\dagger b \\ H_{M-pht} &= (\lambda_{e-pht}a^\dagger c_{D_1}^\dagger c_{D_2} + H.c.) \\ H_{M-phn} &= (\lambda_{e-phn}a^\dagger c_{D_1}^\dagger c_{D_2} + H.c.).\end{aligned}\quad (9)$$

In the above equation,  $\lambda_{e-pht}$  ( $\lambda_{e-phn}$ ) is electron-photon (-phonon) coupling strength. In the left panel of Fig. 1 below we compare the efficiency at maximum power obtained from the model 1 and model 2 in absence of any dephasing and electron-phonon interaction. In the

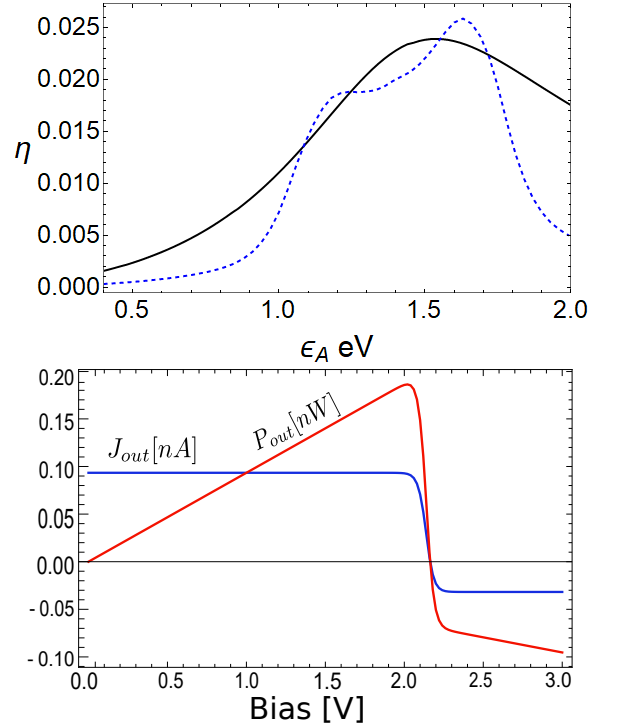

FIG. 1. Left panel: Comparison between the efficiencies at maximum power corresponding to model 1 and model 2; black solid line is from model 1 and blue dashed line corresponds to model 2. Right panel: typical current voltage (IV) characteristic for the HPV cell.

right panel we plot the IV characteristic of model 1 which matches exactly with the IV characteristic corresponding to the model 2 [6]. In both the models mentioned above the quantum transport is not strictly a coherent one since the system is always connected to thermal bath of photons and phonons. In model 1 the system is directly coupled to the thermal baths via Lindblad dissipators whereas, in model 2 corresponding to Ref. [6], the system is first connected to the Bosonic excitations which are subsequently thermalised to their respective baths. One can see from Fig. (1) that  $\eta$  obtained from both the models have same qualitative behaviour, i.e., existence of an optimum acceptor level (value of  $\epsilon_A$ ). The quantitative difference being the number of peaks appearing in

the  $\eta$  vs.  $\epsilon_A$  plot. However, since the maximum of  $\eta$ , obtained from model 2, is appearing at one and only one value of  $\epsilon_A$  we can conclude that both the models are qualitatively and quantitatively similar. With the similarity, explained above, established we have proceeded in the main text with our investigations on the environmental effects on the transport efficiency at maximum power in a single molecule HPV cell.

### III. DEPENDENCE OF THE RESONANT DEPHASING RATE ON ELECTRON-PHONON COUPLING STRENGTH

In Fig. 2 the efficiency at maximum power  $\eta$  and phonon occupation  $n_{phn}$  are plotted as a function of  $\Gamma$  for different values of  $\lambda_{e-ph}$ . From Fig. 2 (a) once can see that value the resonant dephasing rate  $\Gamma_R$  (corresponding to the local minimum of  $\eta$ ) increases with the increase of the value of  $\lambda_{eph}$ . Similarly, the values of  $\Gamma$  at the maxi-

mum of  $n_{phn}$  follow the same trend as that of  $\Gamma_R$ . This implies that with the increase of  $\lambda_{e-ph}$  once needs faster dephasing rate to suppress the available e-ph transport channels. It is worthwhile to note that the magnitude of  $\eta$  at the local minimum increases with the increase of  $\lambda_{e-ph}$  whereas, the magnitude of  $n_{phn}$  decreases with the increase of  $\lambda_{e-ph}$ . This shows that with respect of the variation of  $\lambda_{e-ph}$  value of the local minimum of  $\eta$  is inversely correlated to the maximum of  $n_{phn}$ .

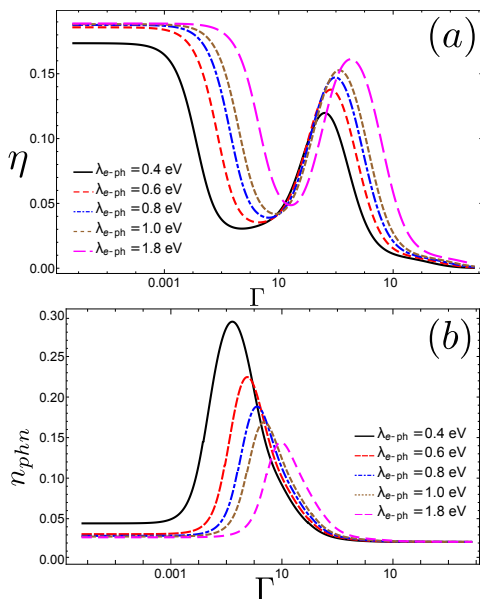

FIG. 2. Plot of (a) efficiency at maximum power  $\eta$  vs dephasing rate  $\Gamma$ , and (b) Plot of phonon occupation  $n_{phn}$  vs dephasing rate  $\Gamma$  for different values of  $\lambda_{e-ph}$ .

- 
- [1] G. Lindblad, On the generators of quantum dynamical semigroups, Commun.Math. Phys. **48**, 119 ((1976)).
  - [2] V. Gorini, A. Kossakowski, and E. C. G. Sudarshan, Completely positive dynamical semigroups of n-level systems, Journal of Mathematical Physics **17**, 821 (1976), <https://aip.scitation.org/doi/pdf/10.1063/1.522979>.
  - [3] H.-P. Breuer and F. Petruccione, Quantum master equations, in *The Theory of Open Quantum Systems* (Oxford University Press, Oxford, 2004) Chap. 3, p. 117.
  - [4] M. Di Ventra, The lindblad equation, in *Electrical Transport in Nanoscale Systems* (Cambridge University Press, 2008) pp. 423–430.
  - [5] A. Purkayastha, A. Dhar, and M. Kulkarni, Out-of-equilibrium open quantum systems: A comparison of approximate quantum master equation approaches with exact results, Phys. Rev. A **93**, 062114 (2016).
  - [6] S. Ajisaka, B. Zunkovic, and Y. Dubi, The molecular photo-cell: Quantum transport and energy conversion at strong non-equilibrium, Scientific Reports **5**, 8312 (2015), article, <https://doi.org/10.1038/srep08312>.
